# Supplementary material for: Acoustic Identification of Ae. aegypti Mosquitoes using Smartphone Apps and Residual Convolutional Neural Networks
Source: arXiv:2306.10091 source file (2023-06-16)
Supplement: Supplementary file 1 [file supplementaryMaterial.tex]

%\documentclass[review]{elsarticle}
\documentclass[3p,preprint]{elsarticle}
\usepackage{hyperref}
%\usepackage{lineno}
%\modulolinenumbers[5]

\usepackage[usenames,dvipsnames]{color}
% \usepackage{cite}
\usepackage{url}
%\usepackage{flushend}
\usepackage[utf8]{inputenc}
\usepackage[T1]{fontenc}

\usepackage[table]{xcolor}

\usepackage{paralist}
% \usepackage{graphicx,url}
\usepackage{amssymb}
\usepackage{subfigure}
\usepackage{amsmath}
\usepackage{graphicx}
% 
\let\proof\relax
\let\endproof\relax
\usepackage{amsthm}
% 
\usepackage{algorithm}
\usepackage{algpseudocode}
% \usepackage{array}
\usepackage{multirow}
\usepackage{xfrac}
% \usepackage{mathtools}
% \usepackage{float}

\hyphenation{mos-qui-to}

\newcommand{\blue}[1]{\textcolor{blue}{#1}} % proposed
\newcommand{\red}[1]{\textcolor{red}{#1}} % to be removed
\newcommand{\magenta}[1]{\textcolor{magenta}{#1}} % warning - requires attention
\newcommand{\N}{\mathbb{N}}
\newcommand{\R}{\mathbb{R}}

\newcommand{\setf}[1]{\fontfamily{phv}\selectfont \tiny{#1}}
\newcommand{\ie}{\emph{i.e.,}\xspace}
\newcommand{\eg}{\emph{e.g.,}\xspace}
\newcommand{\etal}{\emph{et al.}\xspace}
\newcommand{\etc}{\emph{etc.}\xspace}


\begin{document}

\begin{frontmatter}

\author{Marcelo Schreiber Fernandes, Weverton Cordeiro, Mariana Recamonde-Mendoza}
\address{}
%\address{Institute of Informatics, Universidade Federal do Rio Grande do Sul (UFRGS), Porto Alegre, Brazil\\
%      marcelo.schreiber@gmail.com, \{weverton.cordeiro,mrmendoza\}@inf.ufrgs.br}


% \conferenceinfo{SIGCOMM'12,} {August 13--17, 2012, Helsinki, Finland.}
% \CopyrightYear{2012}
% \crdata{978-1-4503-1419-0/12/08}
% \clubpenalty=10000
% \widowpenalty = 10000

%\title{Detecting \emph{Aedes Aegypti} Mosquitoes using Machine Learning-based Audio Analysis}

\title{Detecting \emph{Aedes Aegypti} Mosquitoes through Audio Classification \\with Convolutional Neural Networks \\ \vspace{0.2cm}\textbf{Supplementary Material}}
\end{frontmatter}


\section{Analysis of Fourier Transform Parameters}

\begin{figure}[h]
    \centering
    \includegraphics[width=0.8\textwidth]{img/FFT_Performance_mean_sd.pdf}
    \caption{Average and standard deviation for performance metrics analyzed for each model configuration. }
     \label{fig:eval:fftconfigurationsMean}
\end{figure}

\pagebreak
\vfill
\section{Performance of binary classifier}

\begin{figure}[h]
    \centering
    \includegraphics[width=0.8\textwidth]{img/Binary_Boxplots_c8.pdf}
    \caption{Performance distribution for performance metrics obtained from the binary model..}
    \label{fig:eval:binaryModel1}
\end{figure}


\pagebreak
\vfill
\section{Performance of the multiclass classifier}


\begin{figure}[h]
    \centering
    \includegraphics[width=0.8\textwidth]{img/Multiclass_Boxplots_c8.pdf}
    \caption{Multiclass classification results with model configuration \#8. \emph{Aedes aegypti}, our class of interest, is highlighted in the plot.}
    \label{fig:eval:multiclassc8}
\end{figure}

% \begin{table}[!t]
%     \centering
%     \resizebox{0.48\textwidth}{!}{  
%     \begin{tabular}{c|c|c|c|c} \hline \hline
%          Model config. & No. of bands & No. of frames & Hop length & Window size\\ \hline \hline
%       1 & 20 & 40 & 128 & 1024 \\
%       2 & 40 & 40 & 128 & 1024 \\
%       3 & 60 & 40 & 128 & 1024 \\
%       4 & 80 & 40 & 128 & 1024 \\
%       5 & 60 & 20 & 128 & 1024 \\
%       6 & 60 & 60 & 128 & 1024 \\
%       7 & 60 & 40 & 64 & 1024 \\
%       8 & 60 & 40 & 256 & 1024 \\
%       9 & 60 & 40 & 512 & 1024 \\
%       10 & 60 & 40 & 128 & 512 \\
%       11 & 60 & 40 & 128 & 2048
%       \\ \hline \hline
%     \end{tabular}}
%     \caption{Combination of FFT parameters analyzed in the current work.} %Model configurations in terms of FFT parameters compared in the current work.}
%     \label{tab:eval:list-configurations}
% \end{table}

% \begin{figure}[t]
%     \centering
%     \includegraphics[width=0.47\textwidth]{img/Boxplots_11ModelConfigs.pdf}
%     \caption{Performance distribution for a) accuracy, b) recall, c) precision, and d) F1-measure for the model configurations tested (Table~\ref{tab:eval:list-configurations}). Model configurations \#6 and \#8 were selected for further experiments.}
%     \label{fig:eval:fftconfigurations}
% \end{figure}

% \begin{figure}[h]
%     \centering
%     \includegraphics[width=0.45\textwidth]{img/Performance_summary.pdf}
%     \caption{Average and standard deviation for performance metrics analyzed for each model configuration. }
%      \label{fig:eval:fftconfigurationsMean}
% \end{figure}

% \bibliographystyle{elsarticle-num}
% \bibliography{paper}


\end{document}
